# Supplementary material for: Optimus-2: Multimodal Minecraft Agent with Goal-Observation-Action Conditioned Policy
Source: arXiv:2502.19902 source file (2025-03-11)
Supplement: Supplementary file 1 [file mc-intro.tex]

\begin{figure*}[ht]
    \subfloat[\label{screen_shot:fig1}]{%
      \includegraphics[width=0.5\textwidth]{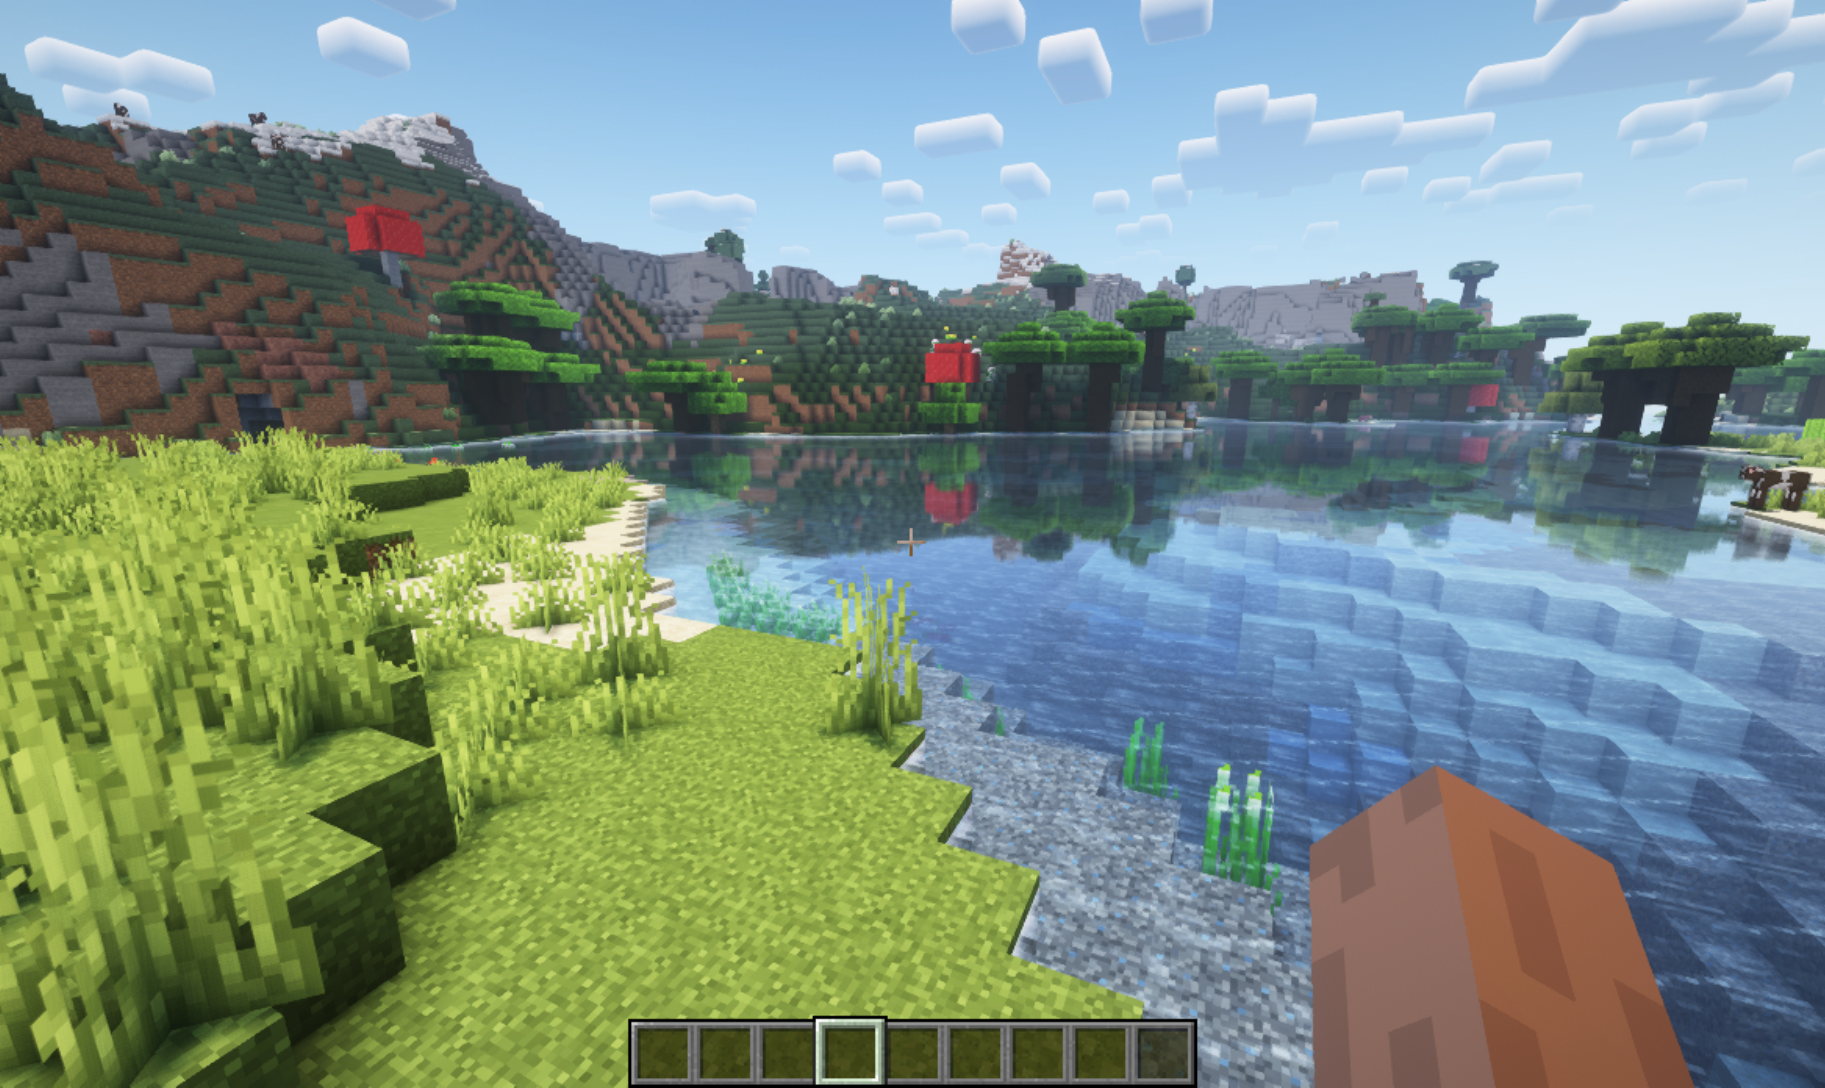}
    }
    \hfill
    \subfloat[\label{screen_shot:fig2}]{%
      \includegraphics[width=0.5\textwidth]{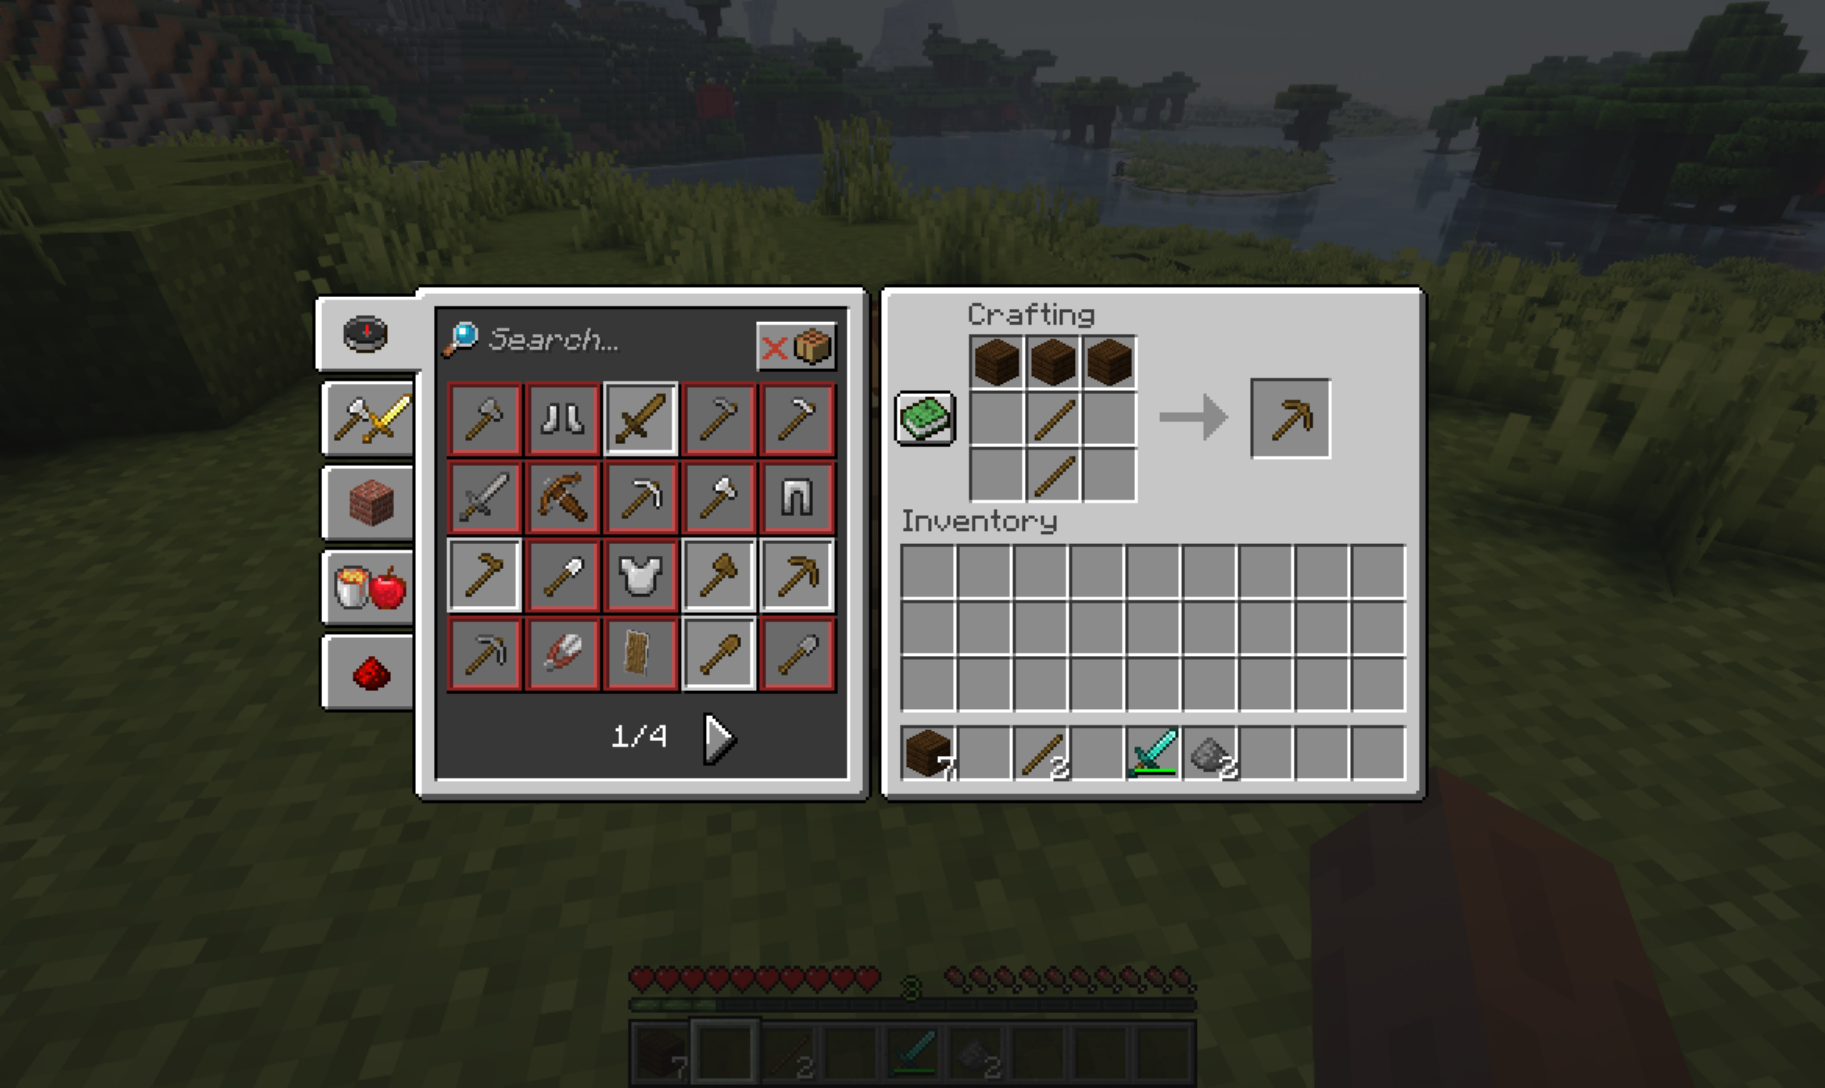}
    }
    \vfill
    \subfloat[\label{screen_shot:fig3}]{%
      \includegraphics[width=0.5\textwidth]{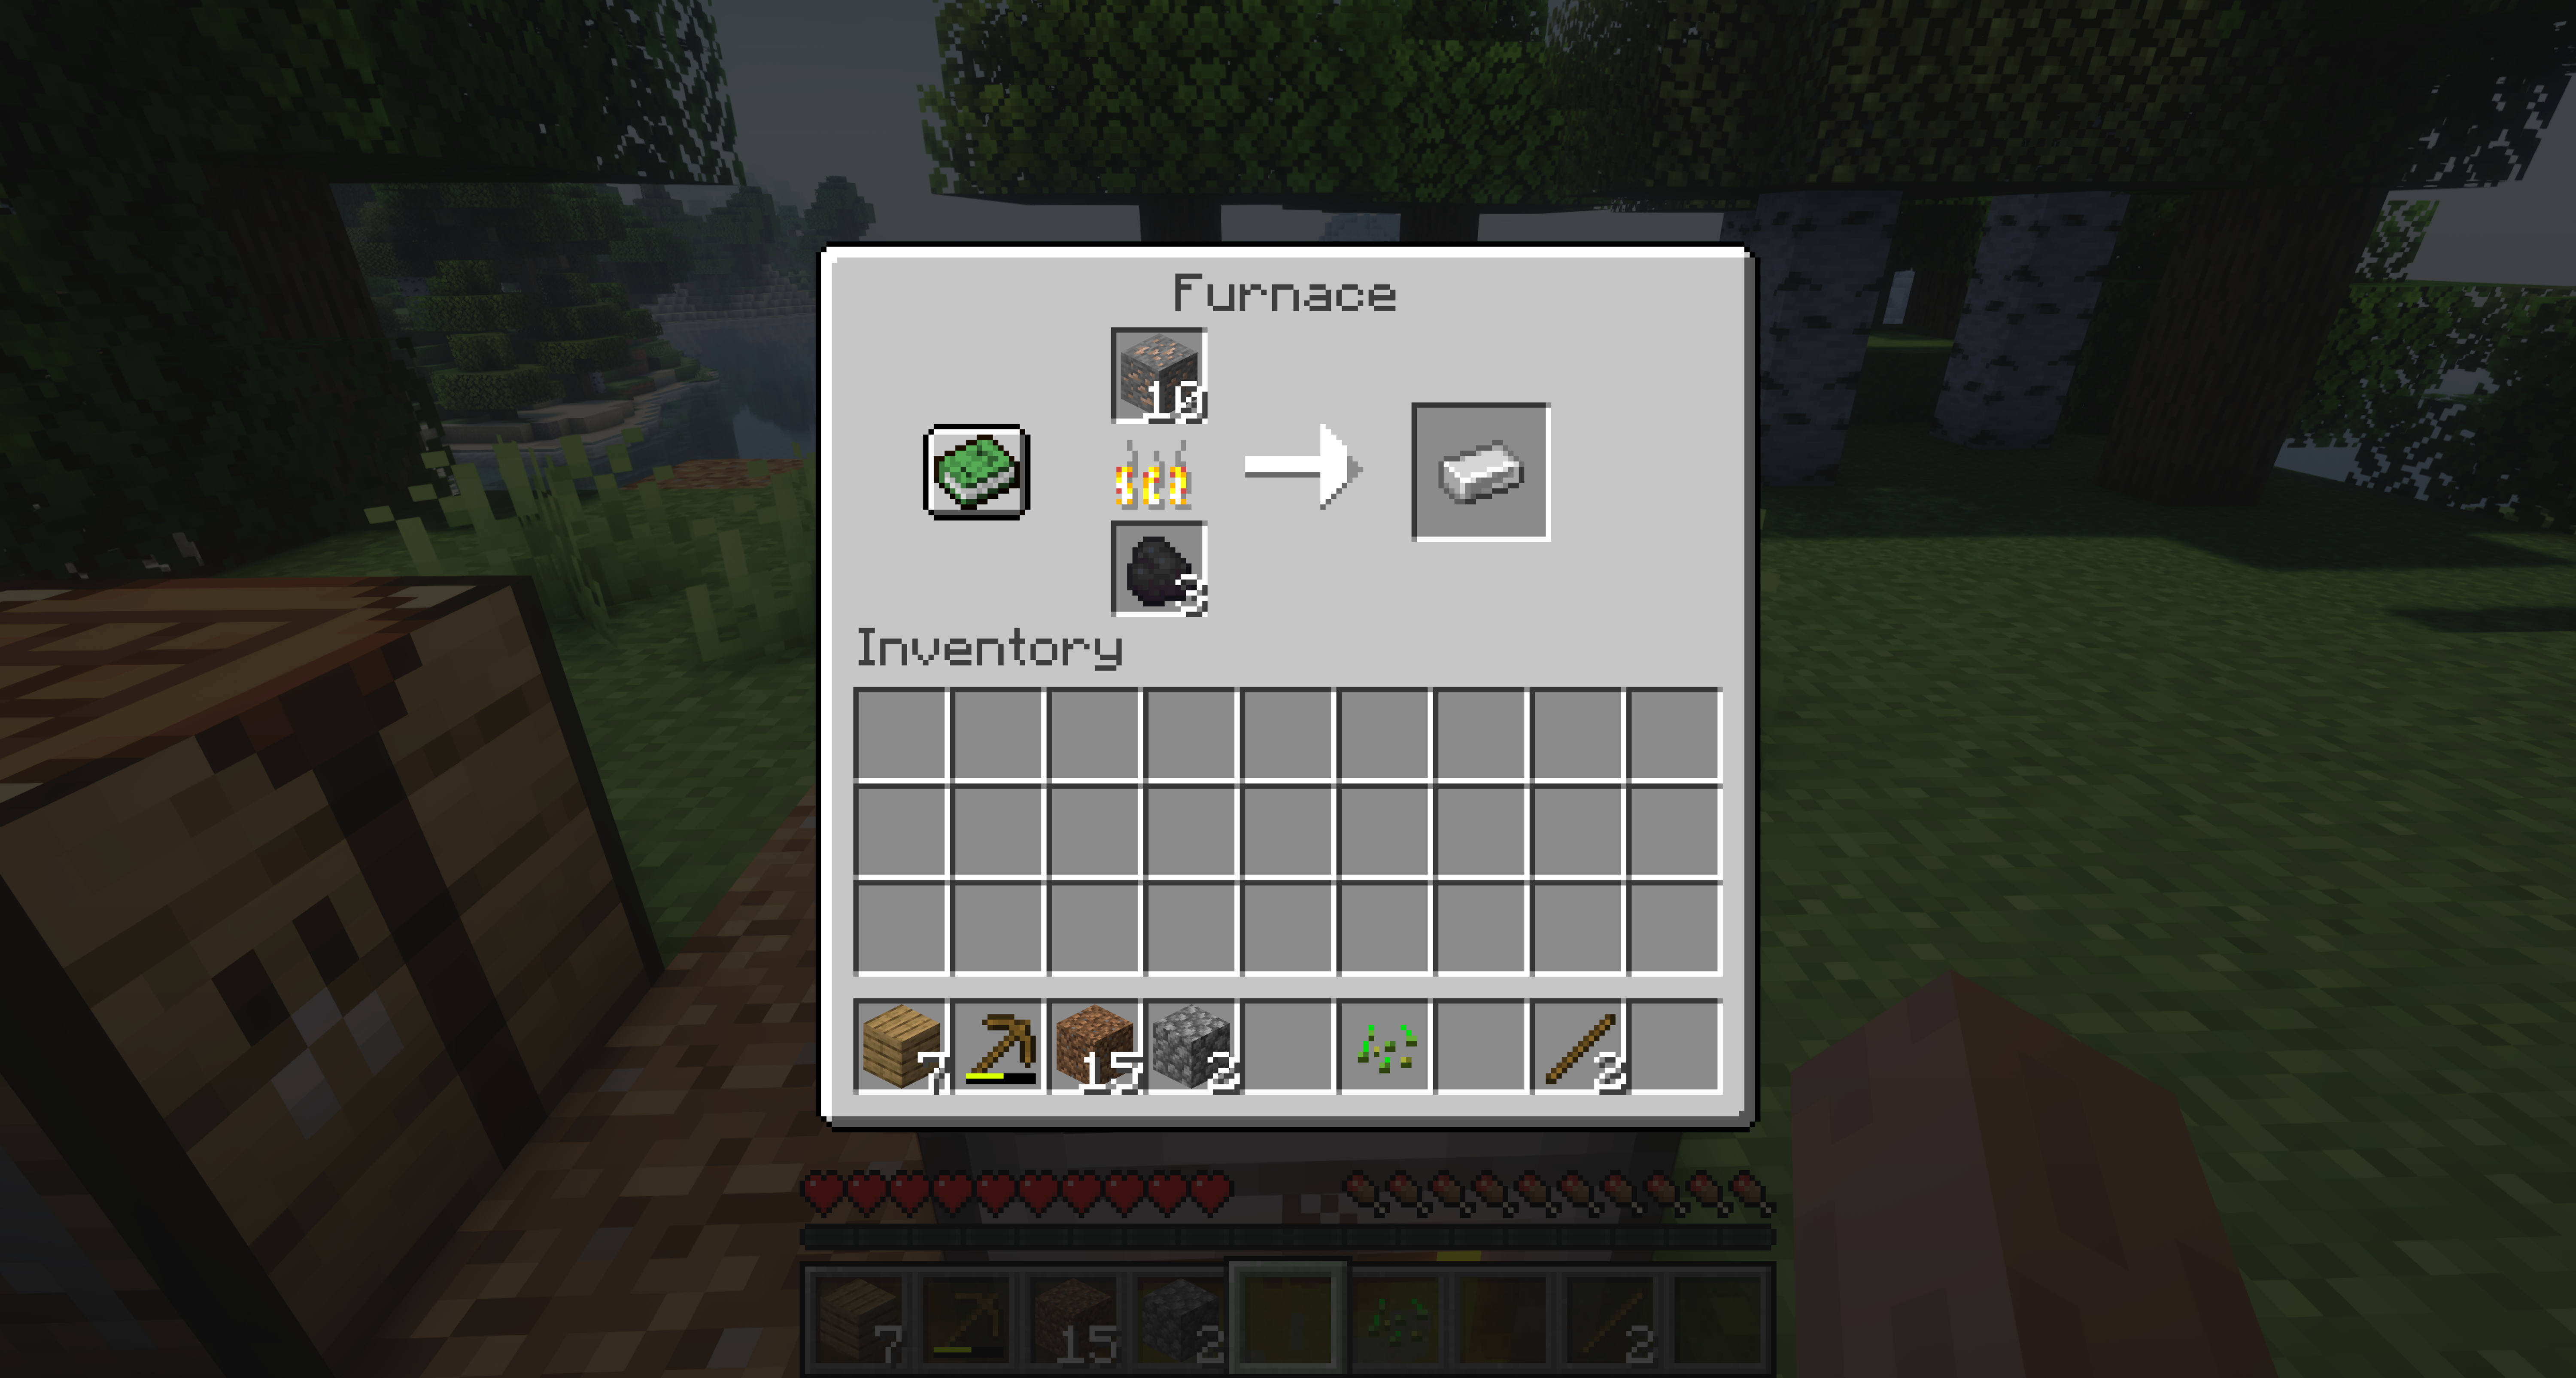}
    }
    \hfill
    \subfloat[\label{screen_shot:fig4}]{%
      \includegraphics[width=0.5\textwidth]{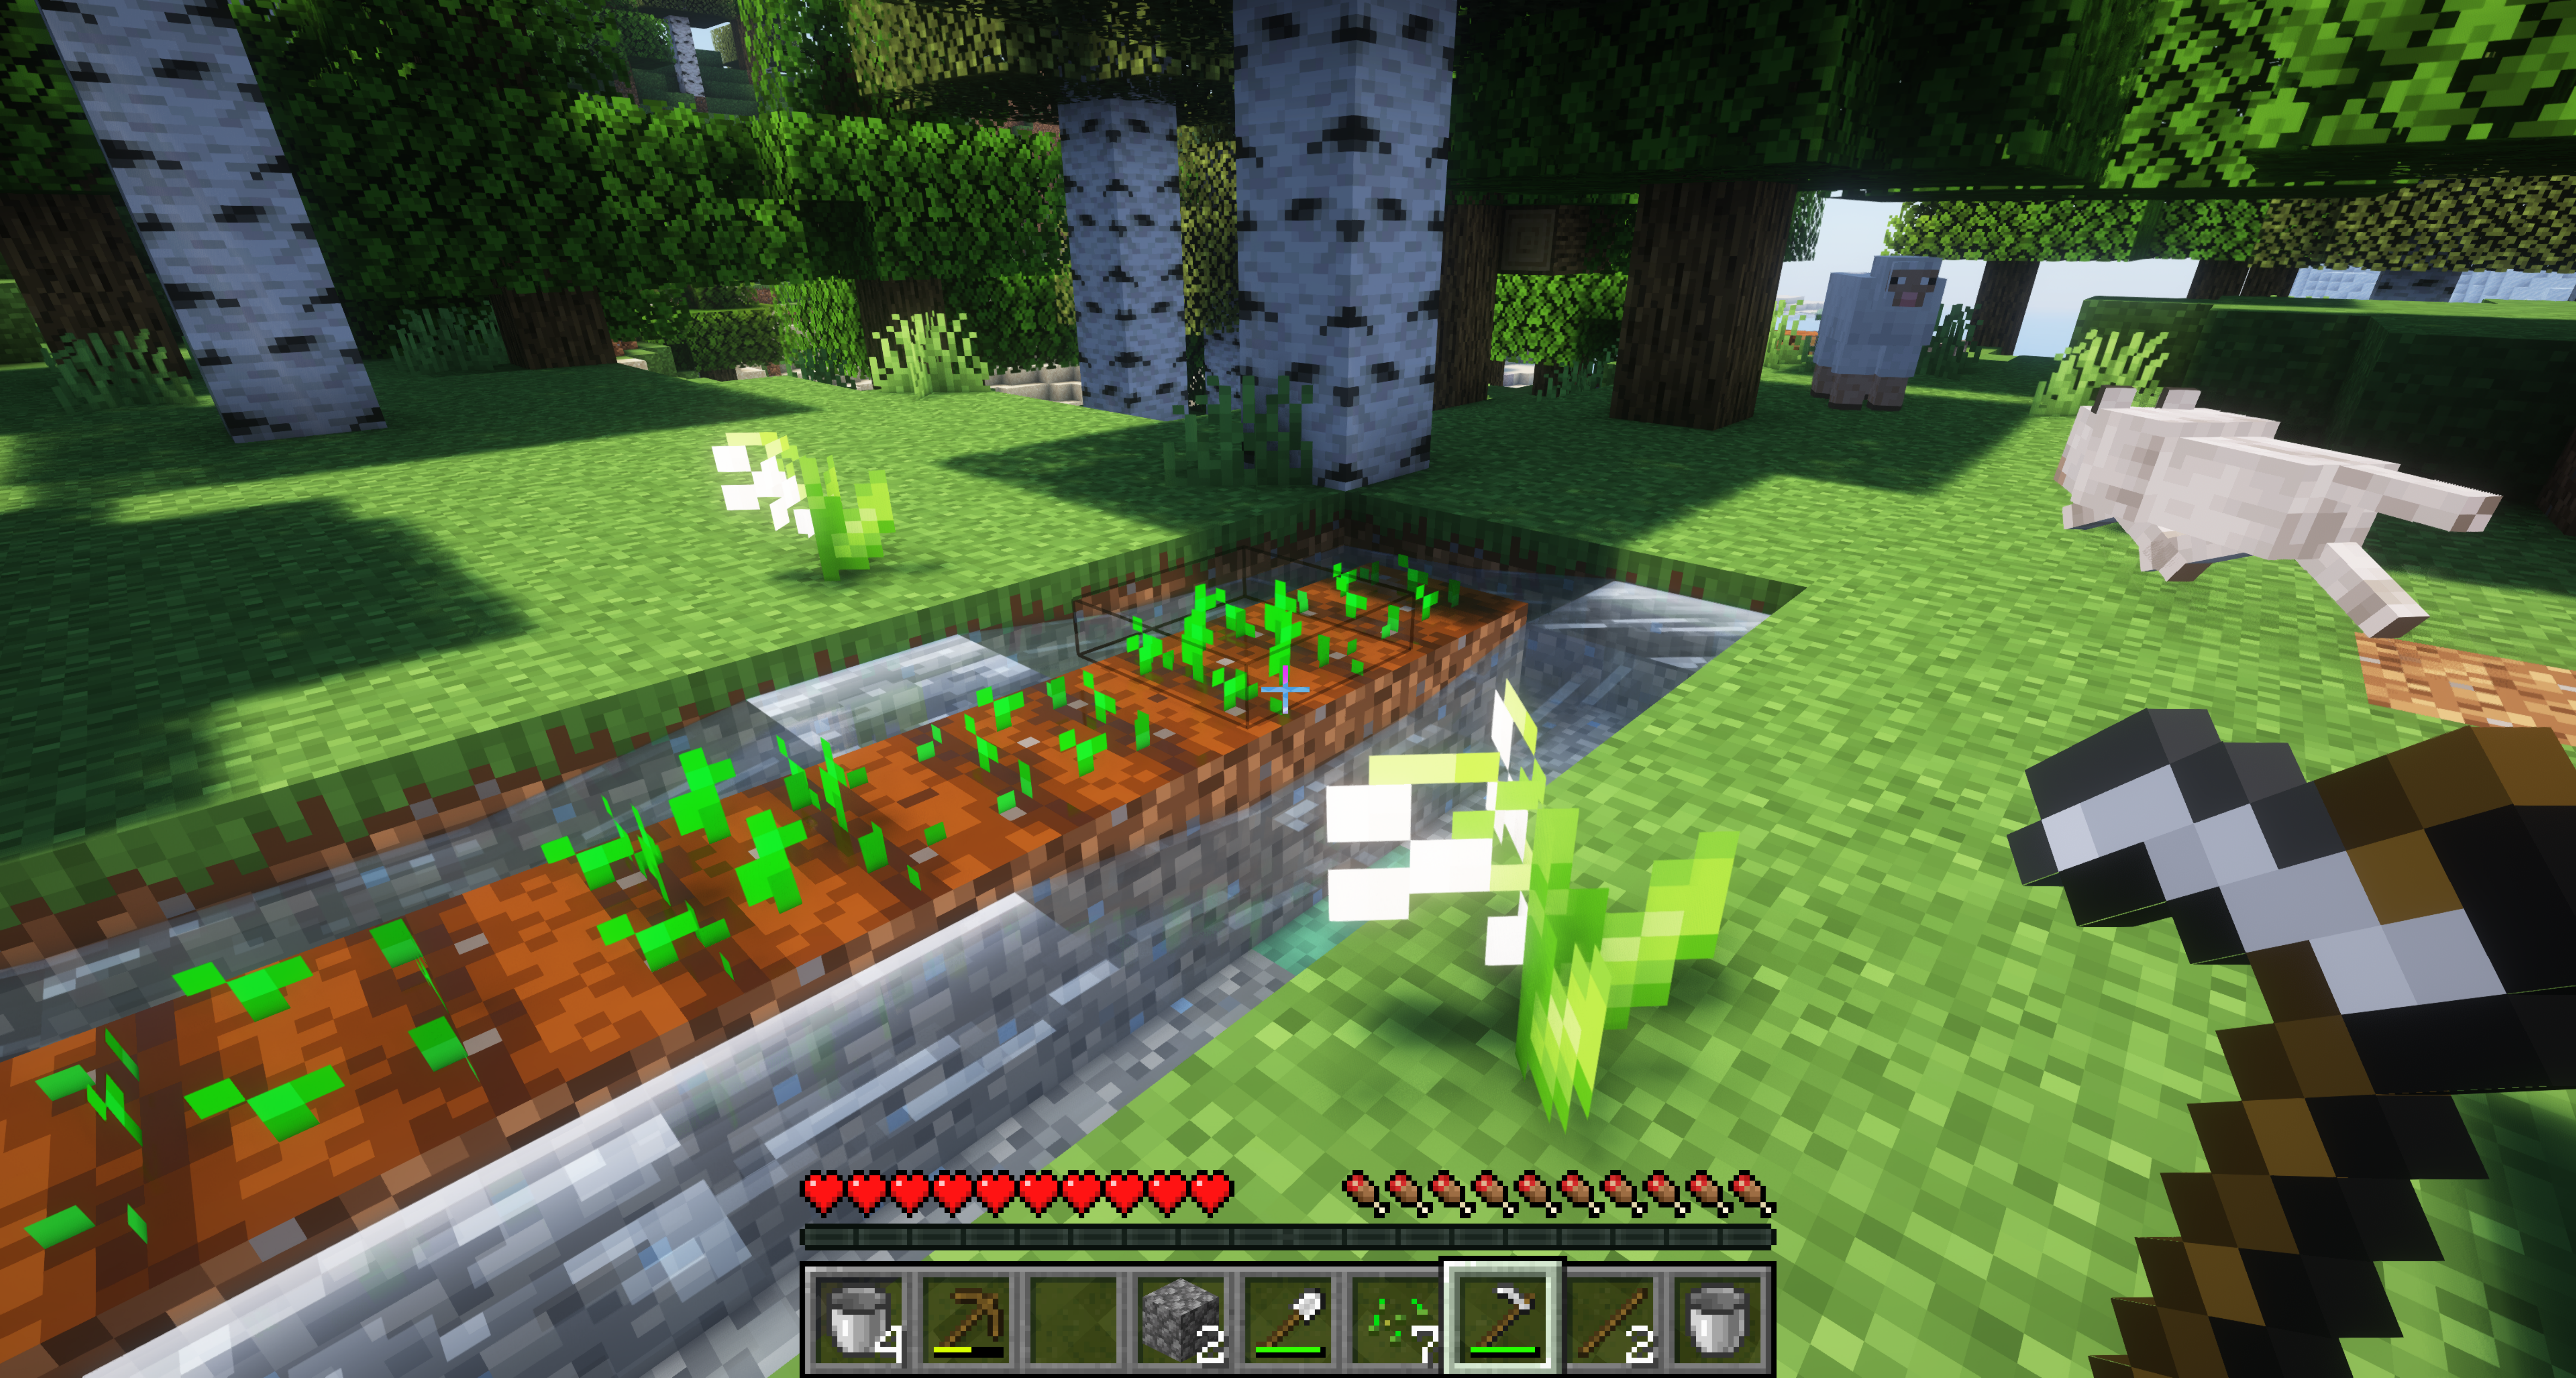}
    }
    \caption{The screenshots in Minecraft. \textbf{(a).} The world has different complex terrains, including plains, river, forest and mine. \textbf{(b).} The agent can use crafting table to craft tools and items with recipes. \textbf{(c).} The agent can use the furnace to smelt ore to obtain precious ingot. \textbf{(d).} The agent can grow wheat near the river.}
    \label{fig:mc-screen-shot}
\end{figure*}
