# Supplementary material for: Optimus-2: Multimodal Minecraft Agent with Goal-Observation-Action Conditioned Policy
Source: arXiv:2502.19902 source file (2025-03-11)
Supplement: Supplementary file 2 [file open_end_ins.tex]

\begin{table*}[!ht]\centering

\begin{tcolorbox}[% 
    breakable,
    ]
\textbf{Plans generated by GPT4V}
\begin{enumerate}
\item First, I need to locate and chop down a couple of trees to collect 4 logs.
\item Next, I should craft these logs into 13 planks.
\item Then, I need to use some of the planks to craft 3 sticks.
\item I will use some of the planks to craft a crafting table.
\item Next, I should craft a wooden pickaxe using some of the planks and sticks.
\item With the wooden pickaxe, I need to find and mine at least 1 coal from a nearby coal deposit or cave.
\item Finally, I can use one stick and one coal to craft a torch.
\end{enumerate}
\tcblower
\textbf{Plans generated by GLM4V}
\begin{enumerate}
\item  Locate and chop down a tree to gather 4 logs.
\item Convert the logs into 13 planks using the crafting menu.
\item Use the planks to craft a crafting table.
\item Craft 3 sticks from the remaining planks.
\item With the crafting table and sticks, craft a wooden pickaxe if one is not already available.
\item Use the wooden pickaxe to dig for coal or kill some Creepers or zombies for coal drops.
\item Once 1 coal is obtained, use the crafting table to combine it with a stick to craft 1 torch.
\end{enumerate}
\end{tcolorbox}
\caption{Open-ended instruction examples of ``Craft a torch''.}
    \label{tab:ins_craft_torch}
\end{table*}

\begin{table*}[!ht]\centering
\begin{tcolorbox}[% 
    breakable,
    ]
\textbf{Plans generated by GPT4V}
\begin{enumerate}
\item First, locate and punch down a tree to acquire 7 logs.
\item Convert these logs into planks to obtain a total of 25 planks.
\item Use some of these planks to craft 5 sticks.
\item Create a crafting table using 4 planks.
\item Craft a wooden pickaxe using 3 planks and 2 sticks.
\item Use the wooden pickaxe to mine 11 cobblestones.
\item Craft a furnace using 8 cobblestones.
\item Craft a stone pickaxe using 3 cobblestones and 2 sticks.
\item Use the stone pickaxe to mine 6 iron ores.
\item Smelt the iron ores in the furnace to create 6 iron ingots.
\item Finally, craft a rail using the iron ingots and sticks.
\end{enumerate}
\tcblower
\textbf{Plans generated by GLM4V}
\begin{enumerate}
\item Locate and gather 7 logs from nearby trees.
\item Use the crafting menu to convert the logs into 25 planks.
\item Craft 5 sticks from the planks.
\item Place down a crafting table to access more crafting recipes.
\item Use the crafting table to craft a wooden pickaxe.
\item With the wooden pickaxe, mine 11 cobblestones from the ground or from stone blocks.
\item Craft a furnace using the cobblestones.
\item Upgrade the wooden pickaxe to a stone pickaxe by crafting it at the crafting table with the cobblestones.
\item Use the stone pickaxe to mine 6 iron ore from the appropriate rock layers.
\item Smelt the 6 iron ore in the furnace to produce 6 iron ingots.
\item Finally, use the crafting table to craft 1 rail using the 6 iron ingots and 1 stick.
\end{enumerate}
\end{tcolorbox}
\caption{Open-ended instruction examples of ``Craft a rail''.}
    \label{tab:ins_craft_rail}
\end{table*}

\begin{table*}[!ht]\centering
\begin{tcolorbox}[% 
    breakable,
    ]
\textbf{Plans generated by GPT4V}
\begin{enumerate}
\item  Start by finding and chopping down trees to collect 9 logs.
\item  Convert the logs into 35 planks using the crafting interface.
\item  Use some of the planks to craft 8 sticks.
\item  Create a crafting table using some of the planks.
\item  Craft a wooden pickaxe using sticks and planks.
\item  Use the wooden pickaxe to mine 19 cobblestone.
\item  Craft a furnace using 8 of the cobblestones.
\item  Use the remaining cobblestone to craft a stone pickaxe.
\item  Mine 3 iron ores using the stone pickaxe.
\item  Smelt the iron ore in the furnace to produce 3 iron ingots.
\item  Craft an iron pickaxe using sticks and iron ingots.
\item  Locate and mine a gold block using the iron pickaxe.
\item  Smelt the gold block in the furnace to get 1 gold ingot.
\item  Finally, use the crafting table to craft a golden shovel using the gold ingot and sticks.
\end{enumerate}
\tcblower
\textbf{Plans generated by GLM4V}
\begin{enumerate}
\item Find and chop down trees to gather 9 logs.
\item Convert the logs into 35 planks using the crafting menu.
\item Craft 8 sticks from the planks.
\item Build a crafting table to expand the crafting options.
\item Use the crafting table to craft a wooden pickaxe with the planks and sticks.
\item With the wooden pickaxe, mine cobblestone until you have a total of 19.
\item Craft a furnace using 8 cobblestone.
\item Use the furnace to smelt the cobblestone into 19 stone, then use the crafting table to craft a stone pickaxe with the stone and sticks.
\item Use the stone pickaxe to mine 3 iron ore.
\item Smelt the iron ore in the furnace to produce 3 iron ingots.
\item Craft an iron pickaxe using the iron ingots and sticks at the crafting table.
\item Use the iron pickaxe to mine a gold block.
\item Smelt the gold block in the furnace to get 1 gold ingot.
\item Finally, use the crafting table to craft the golden shovel using 1 gold ingot and 2 sticks.
\end{enumerate}
\end{tcolorbox}
\caption{Open-ended instruction examples of ``Craft a golden shovel''.}
    \label{tab:ins_craft_golden_shovel}
\end{table*}

\begin{table*}[!ht]\centering
\begin{tcolorbox}[% 
    breakable,
    ]
\textbf{Plans generated by GPT4V}
\begin{enumerate}
\item I have to find a tree to get 9 logs.
\item Next, I have to craft planks.
\item Get sticks.
\item I need a crafting table.
\item I should craft a wooden pickaxe to mine stone.
\item I need 11 cobblestone.
\item I need a furnace.
\item I have to get a stone pickaxe.
\item I need to mine iron ore using the stone pickaxe.
\item Smelt iron ingots in the furnace from the iron ore.
\item Craft an iron pickaxe.
\item Locate a diamond ore and mine it using the iron pickaxe to collect 3 diamonds.
\item Finally, craft a diamond pickaxe using the 3 diamonds and 2 sticks.
\end{enumerate}
\tcblower
\textbf{Plans generated by GLM4V}
\begin{enumerate}
\item  Start by finding trees to gather 9 logs.
\item  Convert the logs into 35 planks.
\item  Craft 8 sticks from the planks.
\item  Build a crafting table to expand crafting options.
\item  Use the crafting table to make a wooden pickaxe.
\item  With the wooden pickaxe, mine 11 cobblestones.
\item  Craft a stone pickaxe using the cobblestones.
\item  Construct a furnace to smelt materials.
\item  Use the stone pickaxe to mine 3 iron ores.
\item  Smelt the iron ores in the furnace to produce 3 iron ingots.
\item Craft an iron pickaxe with the iron ingots.
\item  Locate and mine 3 diamonds, which may require exploring caves or mining deep underground with the iron pickaxe.
\item  Finally, use the crafting table to combine the diamonds and the sticks to craft a diamond pickaxe.
\end{enumerate}
\end{tcolorbox}
\caption{Open-ended instruction examples of ``Craft a diamond pickaxe''.}
    \label{tab:ins_craft_diamond_pickaxe}
\end{table*}

\begin{table*}[!ht]\centering
\begin{tcolorbox}[% 
    breakable,
    ]
\textbf{Plans generated by GPT4V}
\begin{enumerate}
\item  Locate a tree and gather 10 logs.
\item  Convert the logs into 38 planks.
\item  Craft 8 sticks from the planks.
\item  Use some planks to craft a crafting table.
\item  With the crafting table, craft a wooden pickaxe.
\item  Mine cobblestone until you have 12 pieces.
\item  Upgrade your tools by crafting a stone pickaxe.
\item  Construct a furnace using some of the cobblestone.
\item  Use the stone pickaxe to mine 7 iron ore.
\item  Smelt the iron ore in the furnace to produce 7 iron ingots.
\item Craft an iron pickaxe using the iron ingots.
\item  Find and mine redstone using the iron pickaxe to obtain 1 redstone dust.
\item Finally, use the remaining iron ingots and redstone dust at the crafting table to craft a compass.
\end{enumerate}
\tcblower
\textbf{Plans generated by GLM4V}
\begin{enumerate}
\item Locate and gather 10 logs from nearby trees.
\item Convert the logs into 38 planks using the crafting menu.
\item Craft 8 sticks from the planks.
\item Build a crafting table to access more crafting options.
\item Use the crafting table to make a wooden pickaxe.
\item With the wooden pickaxe, mine 12 cobblestones from stone.
\item Craft a stone pickaxe using the cobblestones and the crafting table.
\item Construct a furnace to smelt materials.
\item Use the stone pickaxe to mine 7 iron ores from the appropriate rock formations.
\item Smelt the 7 iron ores in the furnace to produce 7 iron ingots.
\item Craft an iron pickaxe with the iron ingots at the crafting table.
\item Mine for redstone, which can sometimes be found in the ground or in certain stone formations.
\item Once all materials are gathered, use the crafting table to craft a compass with the iron ingot and redstone.
\end{enumerate}
\end{tcolorbox}
\caption{Open-ended instruction examples of ``Craft a compass''.}
    \label{tab:ins_craft_compass}
\end{table*}
