# Supplementary material for: Optimus-2: Multimodal Minecraft Agent with Goal-Observation-Action Conditioned Policy
Source: arXiv:2502.19902 source file (2025-03-11)
Supplement: Supplementary file 3 [file compare_baseline.tex]

\begin{table}[]
\centering
\caption{Statistics for various Minecraft agents.}
\label{tab:compare_baseline}
\resizebox{\textwidth}{!}{%

\begin{tabular}{lcccccccc}
\hline
Agent     & Pub.         & Env.       & Input & Output           & Planning                  & Reflection                & Knowledge                 & Experience                \\ \hline
VPT \cite{vpt}       & NeurIPS' 22 & MineRL     & V     & low-level action &     &     &     &     \\
MineDOJO \cite{fan2022minedojo}  & NeurIPS' 22 & MineDOJO   & T+V   & low-level action &     &     &     &     \\
STEVE-1 \cite{lifshitz2024steve}   & NeurIPS' 23 & MineRL     & T+V   & low-level action &     &     &     &     \\
Voyager \cite{wang2023voyager}   & NeurIPS' 23 & Mineflayer & T+V   & code             & \Checkmark & \Checkmark &     & \Checkmark \\
DEPS \cite{wang2023describe}     & NeurIPS' 23 & MineDOJO   & T+V   & code             & \Checkmark & \Checkmark &     &     \\
GROOT \cite{cai2023groot}    & ICLR' 24    & MineRL     & T+V   & low-level action &     &     &     &     \\
MP5  \cite{qin2023mp5}     & CVPR' 24    & MineDOJO   & T+V   & code             & \Checkmark & \Checkmark &     &     \\
Jarvis-1 \cite{wang2023jarvis} & -            & MineRL      & T+V   & low-level action & \Checkmark & \Checkmark &     & \Checkmark \\
\rowcolor[HTML]{fdf9ea}
Optimus-1 & -            & MineRL     & T+V   & low-level action & \Checkmark & \Checkmark & \Checkmark & \Checkmark \\ \hline
\end{tabular}
}
\end{table}
