# Supplementary material for: Optimus-2: Multimodal Minecraft Agent with Goal-Observation-Action Conditioned Policy
Source: arXiv:2502.19902 source file (2025-03-11)
Supplement: Supplementary file 4 [file eval_task.tex]

% Please add the following required packages to your document preamble:
% \usepackage{graphicx}
\begin{table}[]
\centering
\caption{Setting of 7  groups encompassing 67 Minecraft long-horizon tasks.}
\label{tab:task}
\resizebox{\textwidth}{!}{%

\begin{tabular}{lccccc}
\toprule[1.5pt]
Group    & Task Num. & Example Task                          & Max. Steps & Initial Inventory & Avg. Sub-goal Num. \\ \hline
\includegraphics[width=0.4cm]{picture/logo/wood.pdf} Wooden   & 10        & Craft a wooden axe                    & 3600       & Empty             & 4.60               \\
\includegraphics[width=0.4cm]{picture/logo/cobblestone.pdf} Stone    & 9         & Craft one stone pickaxe               & 7200       & Empty             & 8.78               \\
\includegraphics[width=0.4cm]{picture/logo/iron_ingot.pdf} Iron     & 16        & Craft a iron pickaxe                  & 12000      & Empty             & 12.75              \\
\includegraphics[width=0.4cm]{picture/logo/gold_ingot.pdf} Golden   & 6         & Mine gold and smelt into golden ingot & 36000      & Empty             & 15.83              \\
\includegraphics[width=0.4cm]{picture/logo/readstone.pdf} Redstone & 6         & Craft a piston                        & 36000      & Empty             & 17.50              \\
\includegraphics[width=0.4cm]{picture/logo/diamond.pdf} Diamond  & 7         & Dig down and mine a diamond           & 36000      & Empty             & 15.14              \\
\includegraphics[width=0.4cm]{picture/logo/armor.pdf} Armor    & 13        & Craft one iron helmet                 & 36000      & Empty             & 15.85              \\ 
\bottomrule[1.5pt]
\end{tabular}%
}
\end{table}
