# Supplementary material for: Optimus-2: Multimodal Minecraft Agent with Goal-Observation-Action Conditioned Policy
Source: arXiv:2502.19902 source file (2025-03-11)
Supplement: Supplementary file 5 [file armor.tex]

\begin{table*}[h]
\centering
\caption{The results of Optimus-2 on various tasks in the Armor group. SR denotes success rate.}
\label{tab:armor_result}
\resizebox{0.6\textwidth}{!}{%

\begin{tabular}{cccc}
\toprule[1.5pt]
\textbf{Language Instruction} & \textbf{Sub Goal Num.} & \textbf{SR} & \textbf{Eval Times} \\ \hline
Craft shield             & 14 & 45.16 & 62 \\
Craft iron chestplate    & 14 & 43.86 & 57 \\
Craft iron boots         & 14 & 40.35 & 57 \\
Craft iron leggings      & 14 & 8.57  & 35 \\
Craft iron helmet        & 14 & 47.46 & 56 \\
Craft diamond helmet     & 17 & 9.09  & 33 \\
Craft diamond chestplate & 17 & 7.89  & 38 \\
Craft diamond leggings   & 17 & 5.41  & 37 \\
Craft diamond boots      & 17 & 12.50 & 40 \\
Craft golden helmet      & 17 & 13.89 & 36 \\
Craft golden leggings    & 17 & 12.20 & 41 \\
Craft golden boots       & 17 & 10.26  & 39 \\
Craft golden chestplate  & 17 & 10.00  & 40 \\
\bottomrule[1.5pt]
\end{tabular}%
}
\end{table*}
