# Supplementary material for: Optimus-2: Multimodal Minecraft Agent with Goal-Observation-Action Conditioned Policy
Source: arXiv:2502.19902 source file (2025-03-11)
Supplement: Supplementary file 6 [file diamond.tex]

\begin{table*}[h]
\centering
\caption{The results of Optimus-2 on various tasks in the Diamond group. SR denotes success rate.}
\label{tab:diamond_result}
\resizebox{0.6\textwidth}{!}{%

\begin{tabular}{cccc}
\toprule[1.5pt]
\textbf{Task} & \textbf{Sub Goal Num.} & \textbf{SR}  & \textbf{Eval Times} \\ \hline
Craft a diamond shovel      & 15 & 15.91 & 44 \\
Craft a diamond pickaxe     & 15 & 8.82 & 34 \\
Craft a diamond axe         & 16 & 11.00  & 36 \\
Craft a diamond hoe         & 15 & 15.91  & 44 \\
Craft a diamond sword       & 15 & 11.11 & 36 \\
Dig down and mine a diamond & 15 & 11.42  & 35 \\
Craft a jukebox             & 15 & 13.15 & 38 \\ \bottomrule[1.5pt]
\end{tabular}%
}
\end{table*}
