# Supplementary material for: Optimus-2: Multimodal Minecraft Agent with Goal-Observation-Action Conditioned Policy
Source: arXiv:2502.19902 source file (2025-03-11)
Supplement: Supplementary file 7 [file iron_result.tex]

\begin{table*}[h]
\centering
\caption{The results of Optimus-2 on various tasks in the Iron group. SR denotes success rate.}
\label{tab:iron_result}
\resizebox{0.6\textwidth}{!}{%

\begin{tabular}{cccc}
\toprule[1.5pt]
\textbf{Task} & \textbf{Sub Goal Num.} & \textbf{SR}  & \textbf{Eval Times} \\ \hline
Craft an iron shovel   & 13 & 52.08   & 48 \\
Craft an iron pickaxe  & 13 & 56.00  & 50 \\
Craft an iron axe      & 13 & 48.15  & 54 \\
Craft a stone\_hoe     & 13 & 56.60   & 53 \\
Craft a bucket         & 13 & 45.10   & 51 \\
Craft a hopper         & 14 & 54.90  & 51 \\
Craft a rail           & 13 & 51.02 & 49 \\
Craft an iron sword    & 12 & 56.52  & 46 \\
Craft a shears         & 12 & 48.28 & 58 \\
Craft a smithing table & 12 & 53.33   & 45 \\
Craft a tripwire hook  & 13 & 55.56   & 45 \\
Craft a chain          & 13 & 52.17   & 46 \\
Craft an iron bars     & 12 & 51.06   & 47 \\
Craft an iron nugget   & 12 & 54.55   & 44 \\
Craft a blast furnace  & 14 & 52.27   & 44 \\
Craft a stonecutter    & 13 & 52.27   & 44 \\ \bottomrule[1.5pt]
\end{tabular}%
}
\end{table*}
