# Supplementary material for: Optimus-2: Multimodal Minecraft Agent with Goal-Observation-Action Conditioned Policy
Source: arXiv:2502.19902 source file (2025-03-11)
Supplement: Supplementary file 8 [file redstone.tex]

\begin{table*}[h]
\centering
\caption{The results of Optimus-2 on various tasks in the Redstone group. SR denotes success rate.}
\label{tab:redstone_result}
\resizebox{0.6\textwidth}{!}{%

\begin{tabular}{cccc}
\toprule[1.5pt]
\textbf{Language Instruction} & \textbf{Sub-Goal Num.} & \textbf{SR} & \textbf{Eval Times} \\ \hline
Craft a piston          & 16 & 28.33  & 60 \\
Craft a redstone torch  & 16 & 27.69 & 65 \\
Craft an activator rail & 18 & 25.81 & 62 \\
Craft a compass         & 23 & 28.36 & 67 \\
Craft a dropper         & 16 & 30.30  & 66 \\
Craft a note block      & 16 & 25.40  & 63 \\ \bottomrule[1.5pt]
\end{tabular}%
}
\end{table*}
