# Supplementary material for: Optimus-2: Multimodal Minecraft Agent with Goal-Observation-Action Conditioned Policy
Source: arXiv:2502.19902 source file (2025-03-11)
Supplement: Supplementary file 9 [file stone_result.tex]

\begin{table*}[h]
\centering
\caption{The results of Optimus-2 on various tasks in the Stone group. SR denotes success rate.}
\label{tab:stone_result}
\resizebox{0.6\textwidth}{!}{%

\begin{tabular}{cccc}
\toprule[1.5pt]
\textbf{Task} & \textbf{Sub-Goal Num.} & \textbf{SR} &\textbf{Eval Times} \\ \hline
Craft a stone shovel  & 8  & 89.47 & 57 \\
Craft a stone pickaxe & 10 & 98.00  & 50 \\
Craft a stone axe     & 10 & 94.44  & 54 \\
Craft a stone hoe     & 8  & 95.74  & 47 \\
Craft a charcoal      & 9  & 85.71  & 42 \\
Craft a smoker        & 9  & 90.00  & 40 \\
Craft a stone sword   & 8  & 95.45 & 44 \\
Craft a furnace       & 9  & 94.44  & 36 \\
Craft a torch         & 8  & 89.36  & 47 \\ \bottomrule[1.5pt]
\end{tabular}%
}
\end{table*}
